# Supplementary material for: AlphaCast: A Human Wisdom-LLM Intelligence Co-Reasoning Framework for Time Series Forecasting
Source: arXiv:2511.08947 source file (2026-10-12)
Supplement: Supplementary file 1 [file datasets.tex]

\begin{table*}[htbp]
\centering
\caption{Dataset descriptions. Ex. and En. are abbreviations for the Exogenous variable and Endogenous variable, respectively. The dataset size is organized in (Train, Validation, Test).}
\label{tab:datasets}
\resizebox{\textwidth}{!}{  % 自动缩放表格至页面宽度
\begin{tabular}{l c l l c c}
\hline
\textbf{Dataset} & \textbf{\#Num} & \textbf{Ex. Descriptions} & \textbf{En. Descriptions} & \textbf{Sampling Frequency} & \textbf{Dataset Size} \\
\hline
NP & 2 & Grid Load, Wind Power & Nord Pool Electricity Price & 1 Hour & (10224,1584,3024) \\
PJM & 2 & System Load, SyZonal COMED load & Pennsylvania-New Jersey-Maryland Electricity Price & 1 Hour & (10224,1584,3024) \\
BE & 2 & Generation, System Load & Belgium’s Electricity Price & 1 Hour & (10224,1584,3024) \\
FR & 2 & Generation, System Load & France’s Electricity Price & 1 Hour & (10224,1584,3024) \\
DE & 2 & Wind power, Ampirion zonal load & German’s Electricity Price & 1 Hour & (10224,1584,3024) \\
% BS & 5 & Weather-related Features & Bicycle Rental Count & 1 Hour & (10224,1584,3024) \\
% MOPEX & 4 & Meteorological Forcing Variables & Ddaily Streamflow Discharge & 1 Day & (8544,1344,2544) \\
ETTh1 & 6 & Power Load Feature & Oil Temperature & 1 Hour & (8544,1344,2544) \\
ETTm1 & 6 & Power Load Feature & Oil Temperature & 15 Minutes & (16896,2496,4896) \\
Windy Power & 6 & Meteorological Variables & Power Generation & 15 Minutes & (16896,2496,4896) \\
Sunny power & 6 & Meteorological Variables & Power Generation & 15 Minutes & (16896,2496,4896) \\
\hline
\end{tabular}
}
