# Supplementary material for: AlphaCast: A Human Wisdom-LLM Intelligence Co-Reasoning Framework for Time Series Forecasting
Source: arXiv:2511.08947 source file (2026-10-12)
Supplement: Supplementary file 2 [file feature_overview.tex]

% \begin{table}[t]
%   \centering
%   \caption{Overview of extracted time-series features.}
%   \resizebox{\columnwidth}{!}{
%     \begin{tabular}{l|c}
%       \toprule
%       \textbf{Feature Category} & \textbf{Features} \\
%       \midrule
%       Basic Statistics (7) & basic\_count, basic\_mean, basic\_std, basic\_min, basic\_max, basic\_skew, basic\_kurt \\
%       Spectral Entropy (1) & spectral\_entropy \\
%       \midrule
%       \multirow{4}{*}{\parbox{2.8cm}{\centering tsfeatures (11)}} 
%         & acf\_features: acf1, acf10, diff1\_acf1, diff1\_acf10, diff2\_acf1, diff2\_acf10, season\_acf1 \\
%         & entropy \\
%         & lumpiness \\
%         & flat\_spots \\
%         & crossing\_points \\
%       \midrule
%       Derived Key (1) & seasonal\_strength \\
%       \bottomrule
%     \end{tabular}
%   }
%   \label{tab:feature_overview}
% \end{table}
